# Supplementary material for: Temporal Multiresolution Graph Neural Networks For Epidemic Prediction
Source: arXiv:2205.14831 source file (2022-06-28)
Supplement: Supplementary file 1 [file Appendix.tex]

\section{Appendix}
